# Supplementary material for: LLM Agents can Autonomously Hack Websites
Source: arXiv:2402.06664 source file (2024-02-16)
Supplement: Supplementary file 1 [file appendix.tex]

\section{Further Experimental Details}

% \subsection{Source of Documents}
% 
% TODO

\subsection{Source of Vulnerabilities}

TODO
